# Supplementary material for: AS-Level BGP Community Usage Classification
Source: arXiv:2110.03816 source file (2021-10-07)
Supplement: Supplementary file 1 [file appendix.tex]

\appendix

\section{Appendix}
\label{sec:appendix}

\begin{lstlisting}[language=Python, label={lst:algorithm}, caption={Inference algorithm, iterating over \pcpair pairs by path index $x$, where $path = A_1, A_2, ..., A_n$, and $comm = output(A_1)$.}, float=h, floatplacement=f, mathescape=true, escapechar=\%]
for x=1,...,N:
  # PHASE 1: count %\action%
  for each %\pcpair%:
    assert(cond1)
    t[$A_x$]++ if $A_x$:* in comm
    s[$A_x$]++ if $A_x$:* not in comm
  # PHASE 2: count %\handle%
  for each %\pcpair%:
    assert(cond1 and cond2)
    i[$A_x$]++ if $A_t$:* in comm
    c[$A_x$]++ if $A_t$:* not in comm
\end{lstlisting}

\begin{lstlisting}[language=Python, label={lst:algorithm-alter}, caption={Alternative inference algorithm, iterating over \pcpair pairs without conditions, where $path = A_1, A_2, ..., A_n$, and $comm = output(A_1)$.}, float=h, floatplacement=t, mathescape=true, escapechar=\%]
# INIT
aslist[] = %\silent%|%\ignore%

# PHASE 1: count %\action%
for each %\pcpair%:
  for each i = 1,...,n:
    t[$A_x$]++ if $A_x$:* in comm
    s[$A_x$]++ if $A_x$:* not in comm
# PHASE 2: count %\handle%
for each %\pcpair%:
  for each x = n-1,...,1:
    c[$A_x$]++ if $A_{x+1}$ not in comm
    else:
      i[$A_j$]++ for j in 1,...,$A_{x+1}$
\end{lstlisting}

\begin{table}[H]
\small
  \centering
  \begin{tabular}{|l||r|r|r|r|}
\multicolumn{1}{l}{assigned roles:} & \multicolumn{4}{c}{classification result:}\\\hline
alltf:		& \tagger & \silent & \undecided &   none\\\hline
\tagger		& 69,997 &      0 &         0 &  2,954\\\hline
\multicolumn{5}{l}{}\\\hline
alltc:		& \tagger & \silent & \undecided &   none\\\hline
\tagger		&    766 &      0 &         0 &      0\\
\tagger (hidden) &      0 &      0 &	    0 & 72,185\\\hline
\multicolumn{5}{l}{}\\\hline
random:		& \tagger & \silent & \undecided &   none\\\hline
\tagger		& 22,149 &      0 &         0 &  1,541\\
\silent		&      0 & 21,966 &	    0 &  1,571\\
\tagger (hidden) &      0 &      0 &	    0 & 12,780\\
\silent (hidden) &      0 &      0 &	    0 & 12,944\\\hline
\multicolumn{5}{l}{}\\\hline
random+noise:	& \tagger & \silent & \undecided &   none\\\hline
\tagger		& 21,625 &      0 &        1 &  2,064\\
\silent		&     53 &  3,679 &    17,687 &  2,118\\
\tagger (hidden) &      0 &     12 &	    2 & 12,766\\
\silent (hidden) &      1 &     9 &	    3 & 12,931\\\hline
\multicolumn{5}{l}{}\\\hline
random-p:	    & \tagger & \silent & \undecided &   none\\\hline
\tagger		    &  6,750 &      0 &         0 &  5,876\\
\silent		    &      0 & 13,445 &         0 & 11,983\\
\selective	    &  2,351 &  3,538 &       837 &  5,984\\
\tagger (hidden)    &      0 &      0 &         0 &  5,562\\
\silent (hidden)    &      0 &      0 &	        0 & 11,082\\
\selective (hidden) &      0 &      0 &         0 &  5,543\\\hline
\multicolumn{5}{l}{}\\\hline
random-pp:	   & \tagger & \silent & \undecided &   none\\\hline
\tagger		   &  2,163 &      0 &         0 &  10,463\\
\silent		   &      0 &  4,429 &         0 & 20,999\\
\selective	   &  1,301 &    713 &       134 &   10,562\\
\tagger (hidden)	   &      0 &      0 &         0 &  5,562\\
\silent (hidden)    &      0 &      0 &	       0 & 11,082\\
\selective (hidden) &      0 &  0 &         0 & 5,543\\\hline
  \end{tabular}
  \caption{Assigned roles vs. classification results: Confusion Matrices for \action behavior per scenario.}
  \label{tab:confusion-action}
\end{table}

\begin{table}[H]
\small
  \centering
  \begin{tabular}{|l||r|r|r|r|}
\multicolumn{1}{l}{assigned roles:} & \multicolumn{4}{c}{classification result:}\\\hline
alltf: 	   & \ignore & \cleaner & \undecided &   none\\\hline
\ignore		   &  10,427 &        0 &          0 &  2,104\\
\ignore (leaf)	   &       0 &        0 &          0 & 60,420\\\hline
\multicolumn{5}{l}{}\\\hline
alltc: 	   & \ignore & \cleaner & \undecided &   none\\\hline
\cleaner	  &       0 &      578 &          0 &    124\\
\cleaner (hidden) &       0 &        0 &          0 & 11,829\\
\cleaner (leaf)	  &       0 &        0 &          0 & 60,420\\\hline
random: 	   & \ignore & \cleaner & \undecided &   none\\\hline
\ignore		   &   2,400 &        0 &          0 &  1,091\\
\cleaner	   &       0 &    2,433 &          0 &  1,106\\
\ignore (hidden)   &       0 &        0 &          0 &  2,750\\
\cleaner (hidden)  &       0 &        0 &          0 &  2,750\\
\ignore (leaf)	   &       0 &        0 &          0 & 30,335\\
\cleaner (leaf)    &       0 &        0 &          0 & 30,085\\\hline
\multicolumn{5}{l}{}\\\hline
random+noise: 	   & \ignore & \cleaner & \undecided &   none\\\hline
\ignore		   &   2,294 &        0 &         63 &  1,134\\
\cleaner	   &       1 &      738 &      1,647 &  1,153\\
\ignore (hidden)   &       0 &        2 &          2 &  2,746\\
\cleaner (hidden)  &       0 &        1 &          0 &  2,750\\
\ignore (leaf)	   &       0 &        0 &          0 & 30,335\\
\cleaner (leaf)    &       0 &        0 &          0 & 30,085\\\hline
\multicolumn{5}{l}{}\\\hline
random-p:	   & \ignore & \cleaner & \undecided &   none\\\hline
\ignore		   &     925 &       75 &        266 &  1,666\\
\cleaner	   &       0 &    1,355 &          0 &  1,663\\
\ignore (hidden)   &       0 &       52 &          0 &  3,265\\
\cleaner (hidden)  &       0 &       47 &          0 &  3,217\\
\ignore (leaf)	   &       0 &        0 &          0 & 30,480\\
\cleaner (leaf)    &       0 &        0 &          0 & 29,940\\\hline
\multicolumn{5}{l}{}\\\hline
random-pp:	   & \ignore & \cleaner & \undecided &   none\\\hline
\ignore		   &     221 &       72 &        279 &  2,341\\
\cleaner	   &       0 &      610 &          0 &  2,386\\
\ignore (hidden)   &       0 &       14 &          0 &  3,322\\
\cleaner (hidden)  &       0 &       19 &          0 &  3,267\\
\ignore (leaf)     &       0 &        0 &          0 & 30,480\\
\cleaner (leaf)    &       0 &        0 &          0 & 29,940\\\hline
  \end{tabular}
  \caption{Assigned roles vs. classification results: Confusion Matrices for \handle behavior per scenario.}
  \label{tab:confusion-handle}
\end{table}
